# Supplementary material for: A Novel ICD Coding Method Based on Associated and Hierarchical Code Description Distillation
Source: arXiv:2404.11132 source file (2024-08-31)
Supplement: Supplementary file 1 [file 07_appendix.tex]

\section{Appendix}
\label{sec:appendix}

\subsection{Case Study}
\begin{figure}[h]
	\centering
	\includegraphics[scale=0.44]{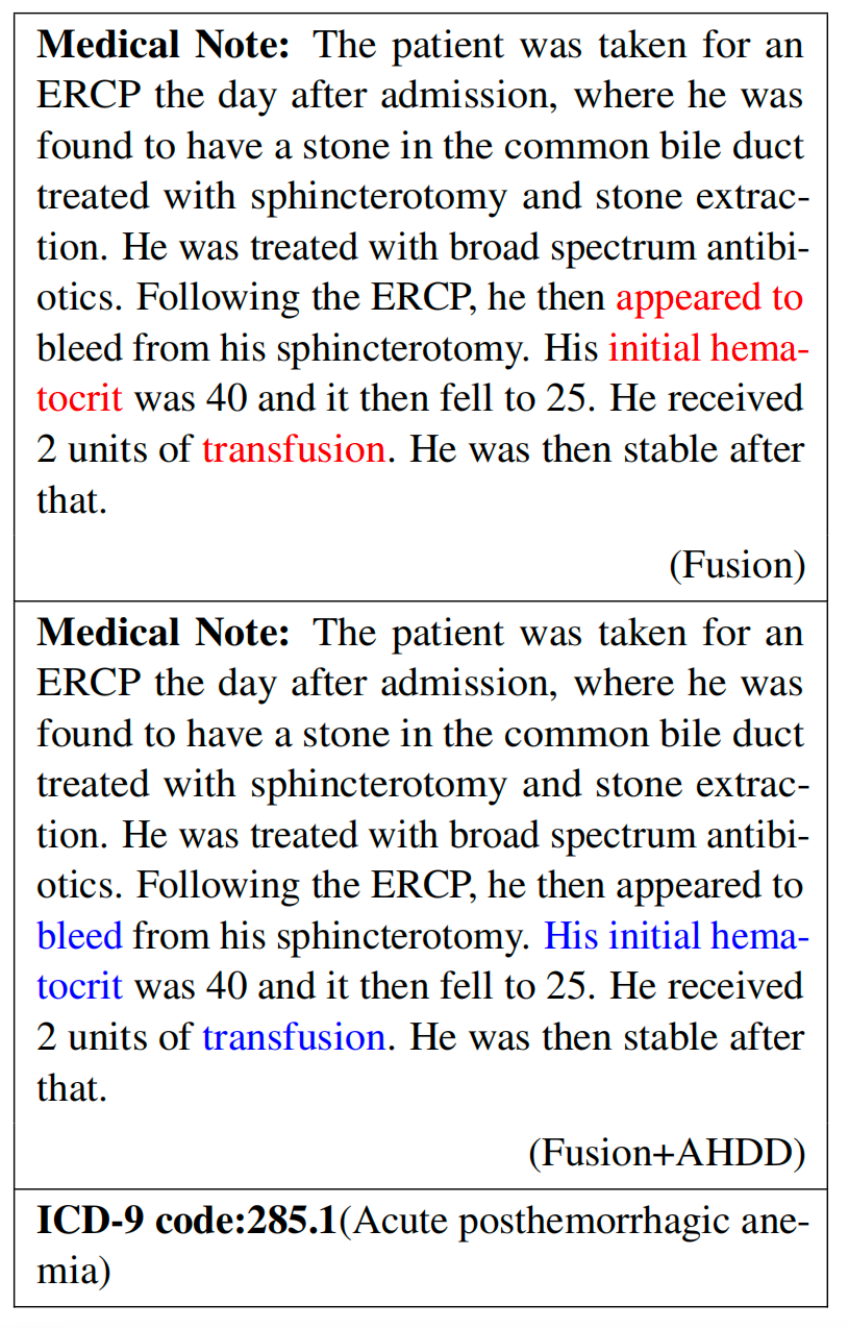} 
	\caption{The attention distribution visualization over a medical note with a medical code for Fusion and its counterparts under AHDD framework. We calculate the attention score over hidden states encoded, and highlight the highly weighted words.}
	\label{Figure visual}
\end{figure}
\textbf{Visualization of Attention Distribution}
To further explore the proposed framework's ability to capture relevant information, we present a visualization of the attention distribution over a medical note. This visualization compares Fusion and its counterparts within our AHDD framework, as illustrated in \figref{Figure visual}.

It can be observed that Fusion only captures scattered label-related words like "\textit{appeared to}", "\textit{initial hematocrit}" and "\textit{transfusion}" for inferring "\textit{anemia}", while it fails to find valid relevant evidence for inferring "\textit{Acute posthemorrhagic anemia}". In contrast, the AHDD framework, which utilizes associated and hierarchical code description distillation, successfully identifies the crucial word "\textit{bleed}" to infer ICD code 285.1. Therefore, through the distillation , the model can more effectively capture significant words and avoid improper code assignments.

\subsection{Experiment About Rare Codes}
\begin{figure*}[h]
    \centering
    \begin{minipage}[b]{\linewidth}
        \centering
        \includegraphics[width=.3\linewidth]{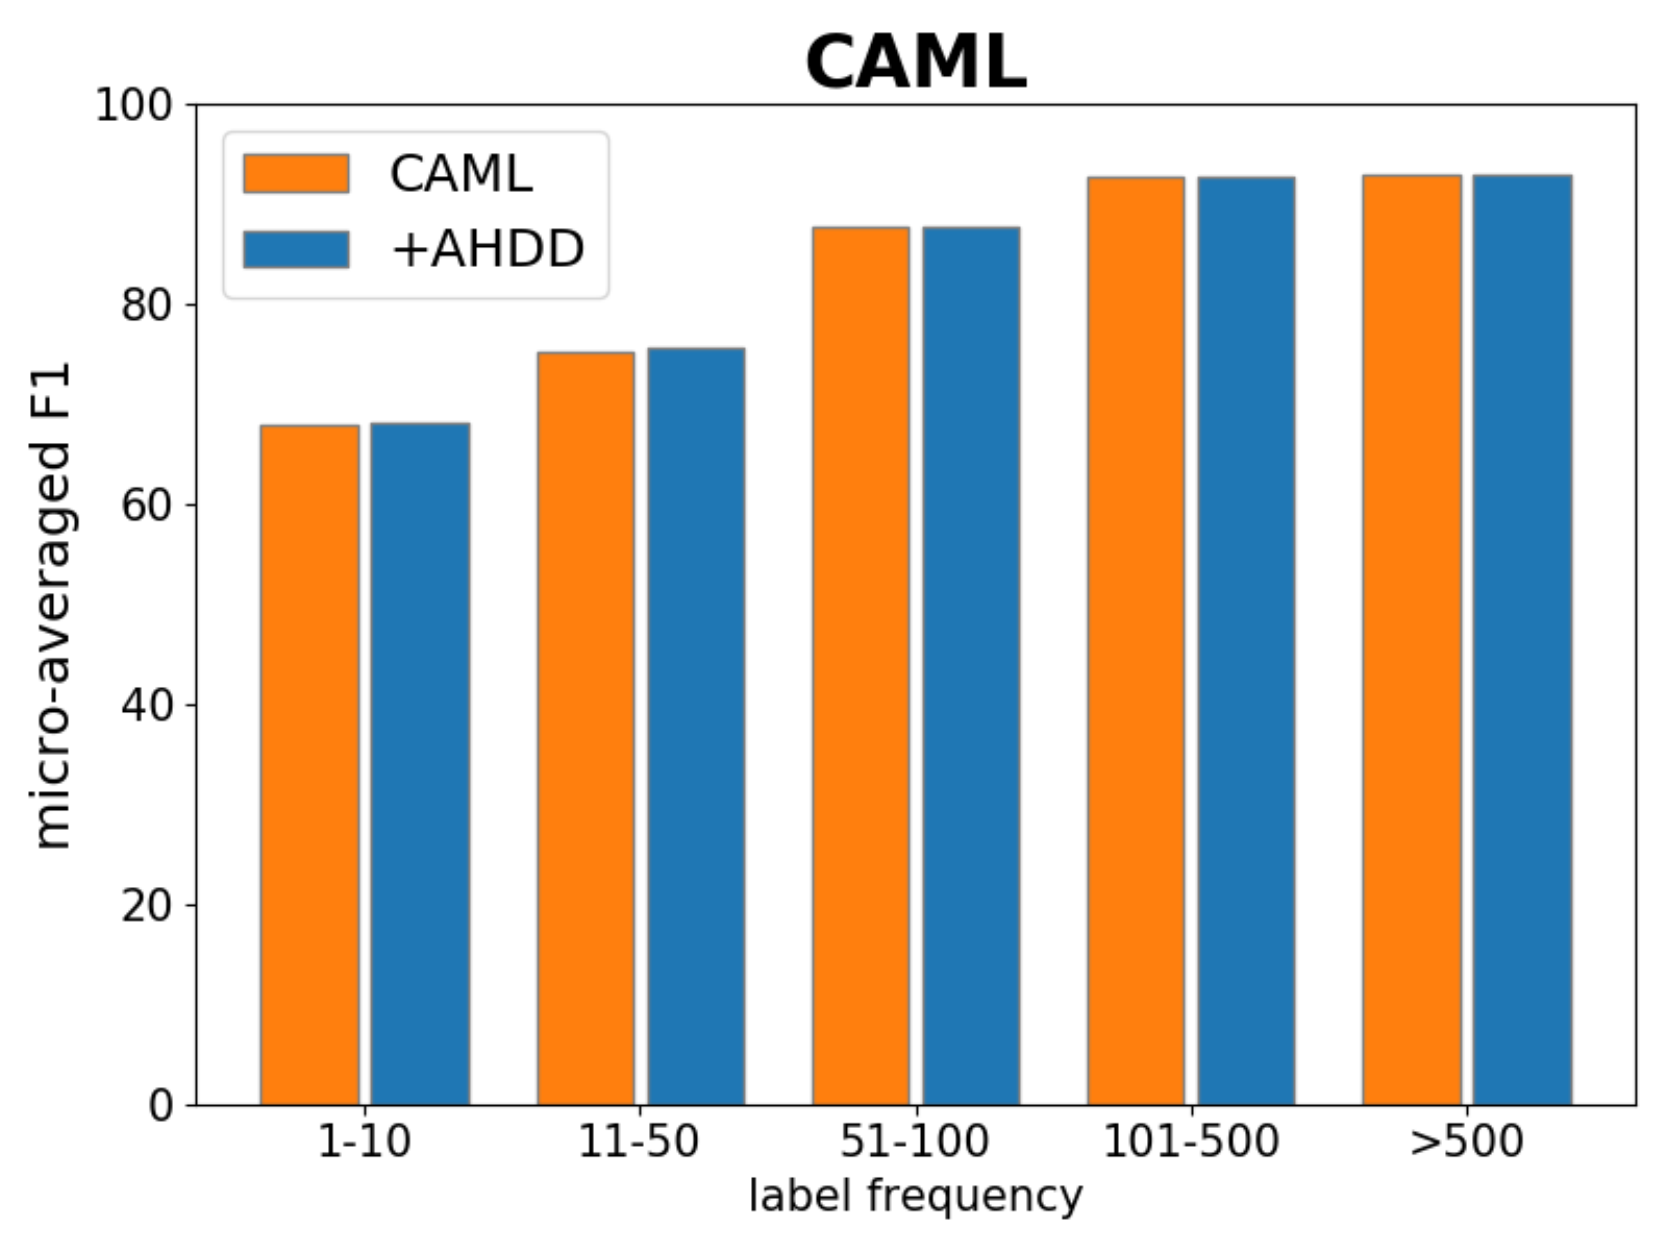}
        \includegraphics[width=.3\linewidth]{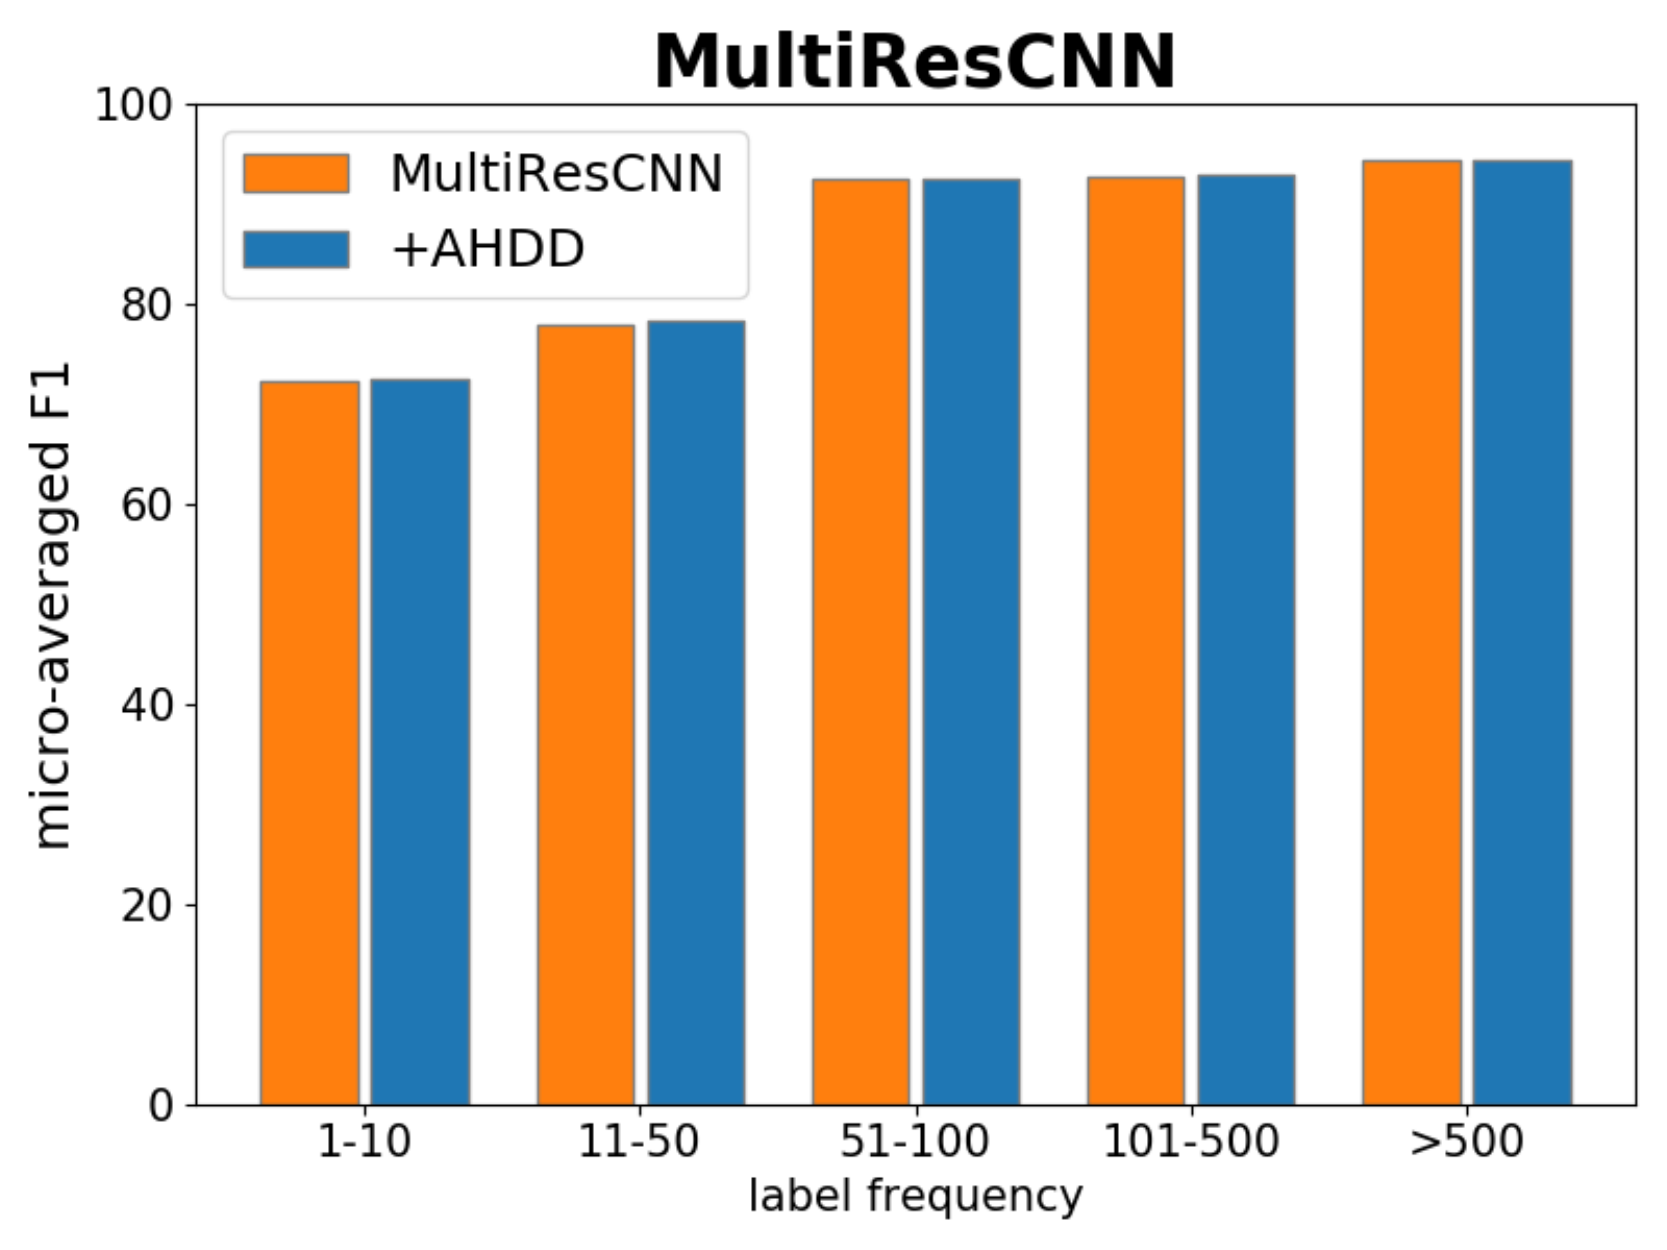}
        \includegraphics[width=.3\linewidth]{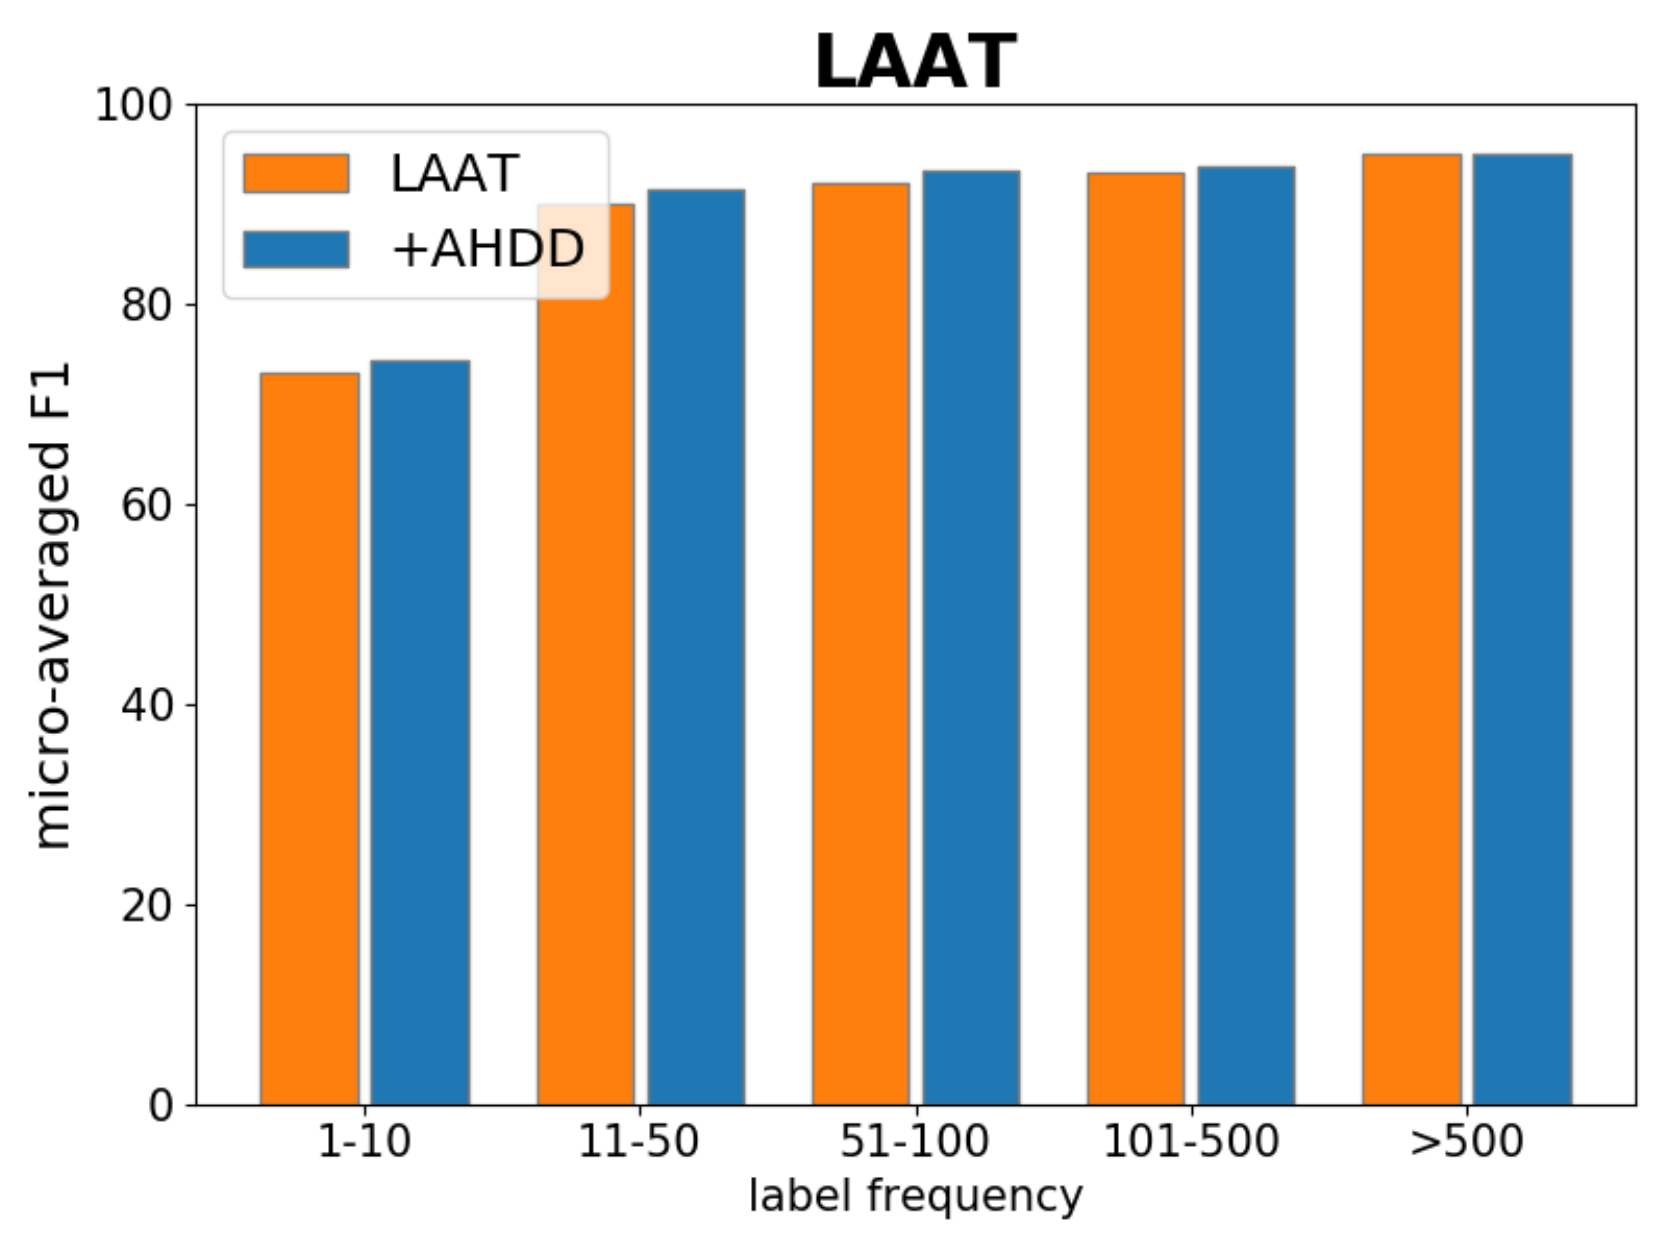}
    \end{minipage}
    \centering
    \begin{minipage}[b]{\linewidth}
        \centering
        \includegraphics[width=.3\linewidth]{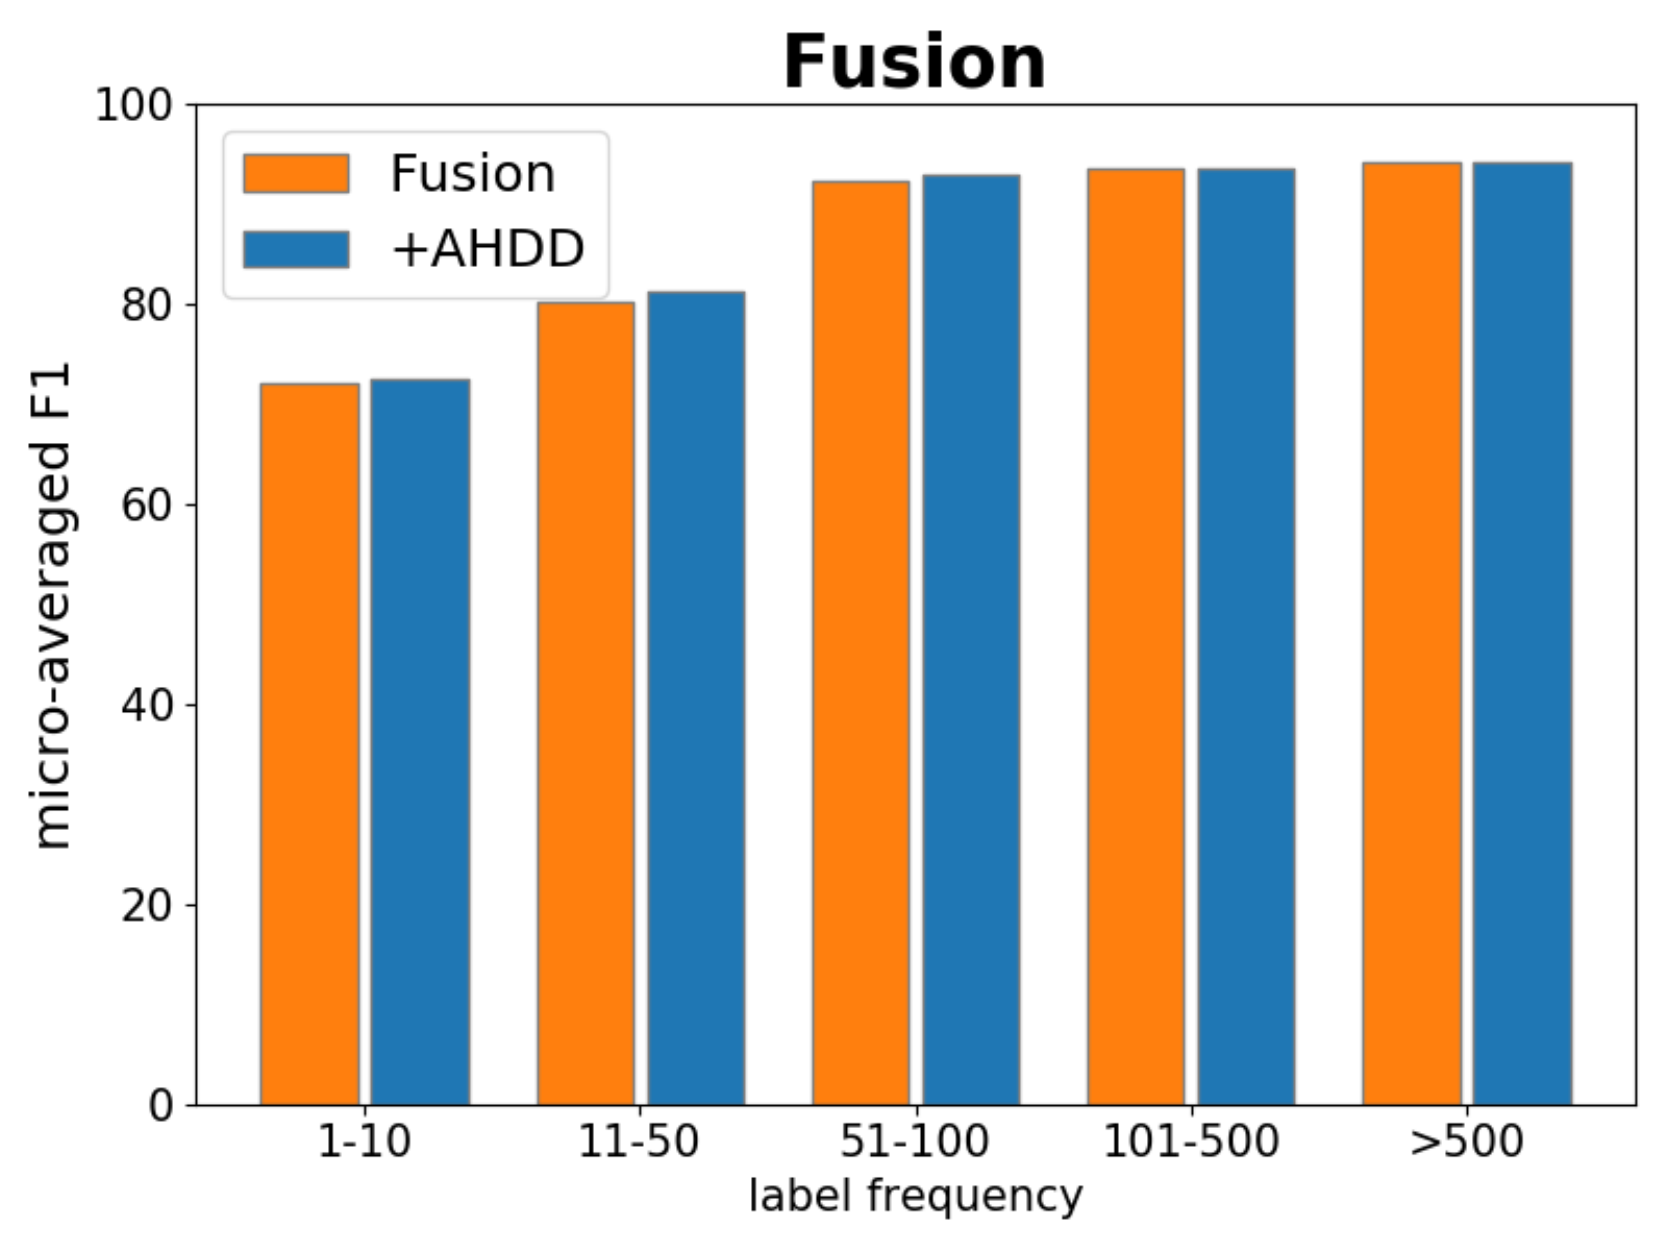}
        \includegraphics[width=.3\linewidth]{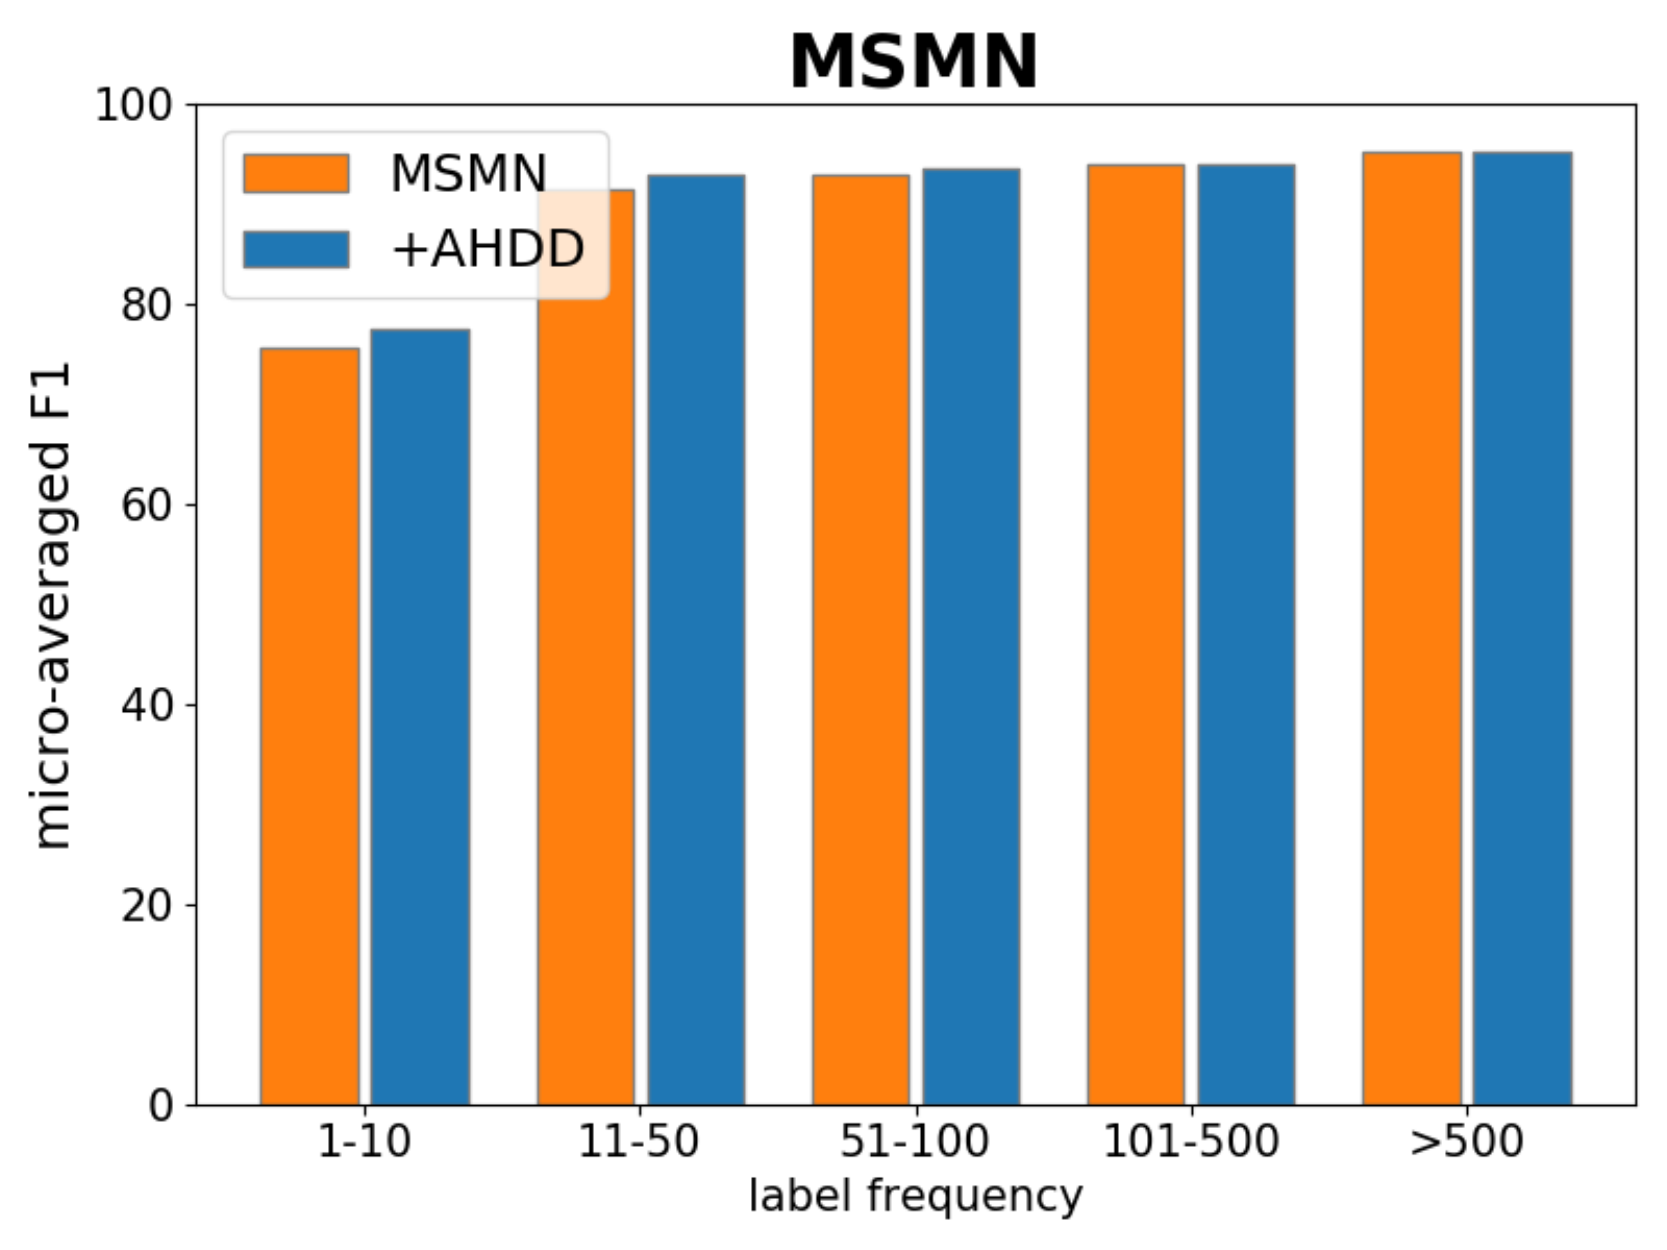}
        \includegraphics[width=.3\linewidth]{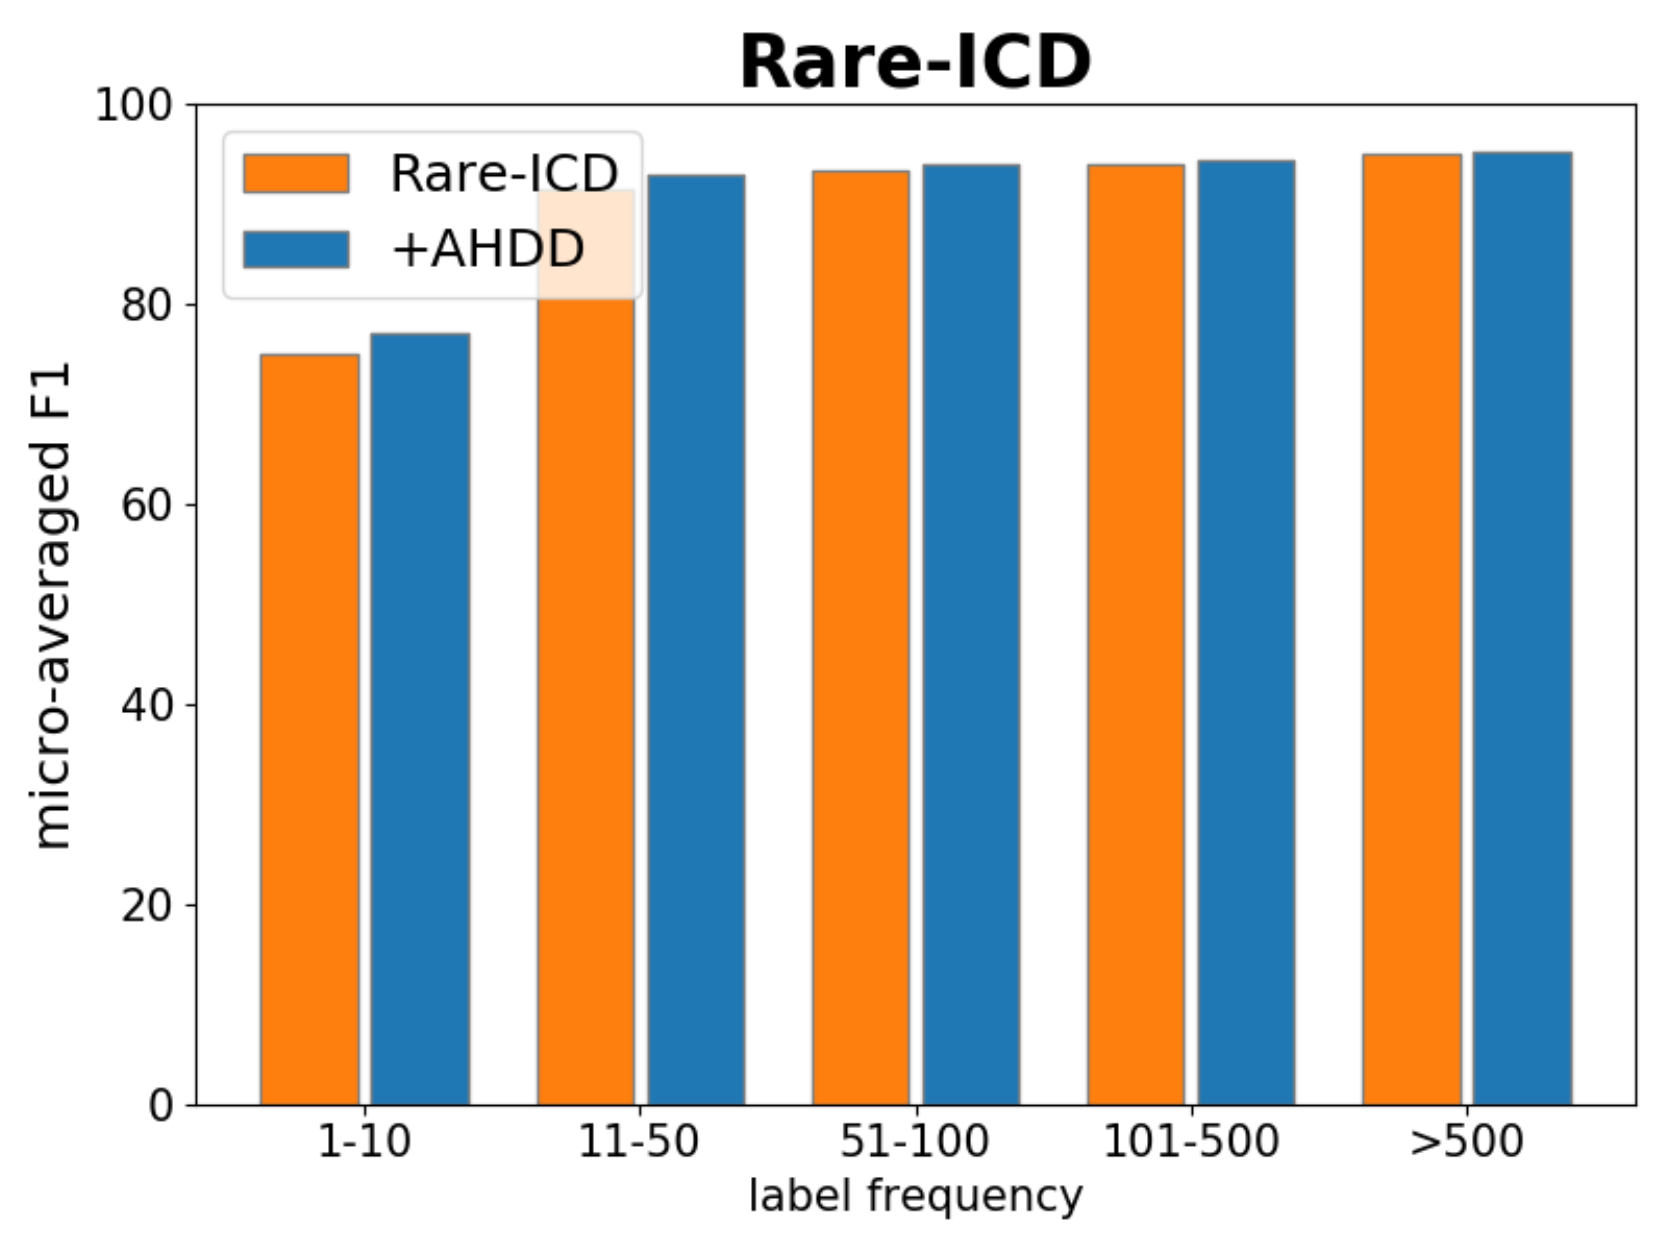}
    \end{minipage}

    \caption{Micro-averaged F1 for the label frequency groups for CAML, MultiResCNN, LAAT, Fusion, MSMN and Rare-ICD models. The x-axis represents the groups based on label frequency, while the y-axis shows the micro-averaged F1 for each of these groups. }
	\label{Figure 4}
\end{figure*}
The proposed method also addresses the issue of rare codes. We have adopted the data split methodology proposed by \cite{knowledge}, dividing medical codes into five groups: [1,10], [11,50], [51,100], [101,500], and [501, +\( \infty \)] based on frequency in the dataset and calculating the macro-averaged F1 for each group. The results, as summarized in \figref{Figure 4}., demonstrate the effectiveness of our method across different frequency groups.

\subsection{Ablation Study On Other Methods}
\input{table/ablation_result other}
To comprehensively assess the impact of each individual component, we carried out a series of ablation experiments on other methods. The results of these experiments are detailed in Table \ref{Table ablation other}.
